# Supplementary material for: A generalized and adaptable tensor-contraction-based cluster expansion formalism for multicomponent solids
Source: arXiv:2509.04686 ancillary file (2025-10-22)
Supplement: Supplementary file 1 [file supplementary.pdf]

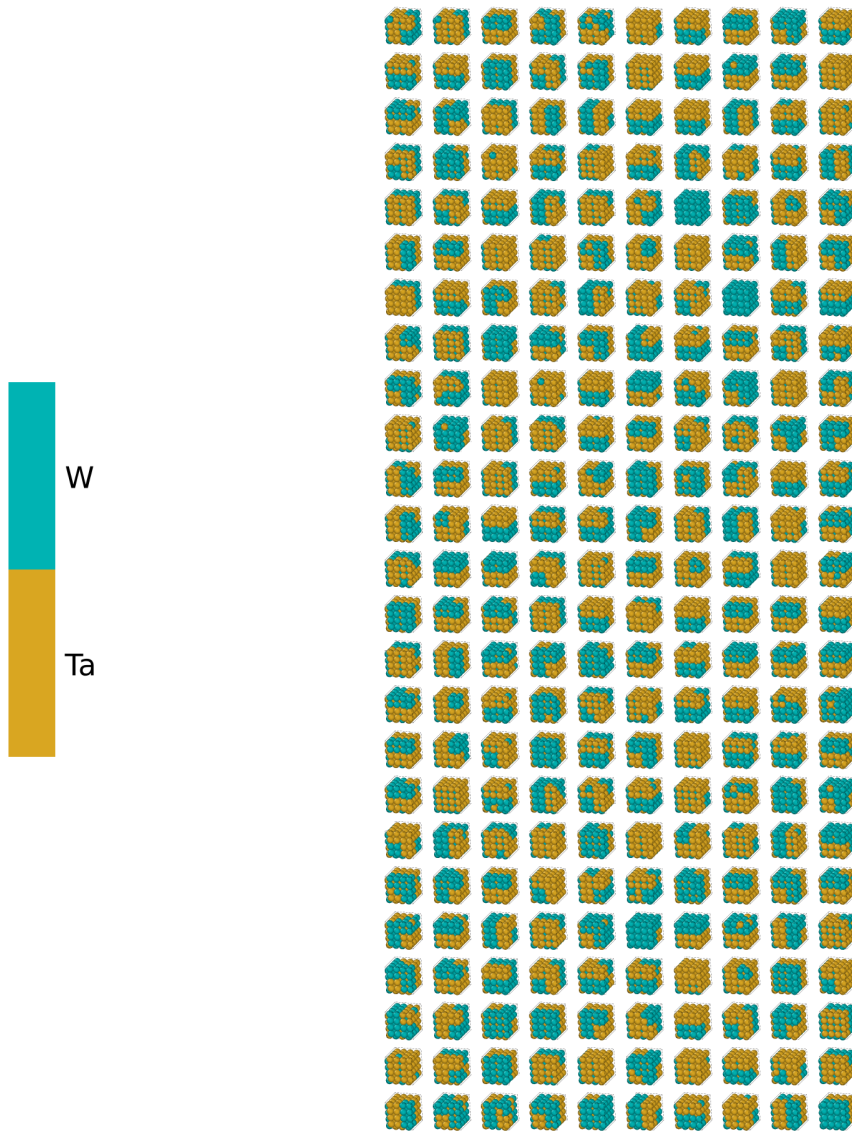

Figure 1: Full TaW training set, generated via a genetic algorithm starting from ordered seeds.

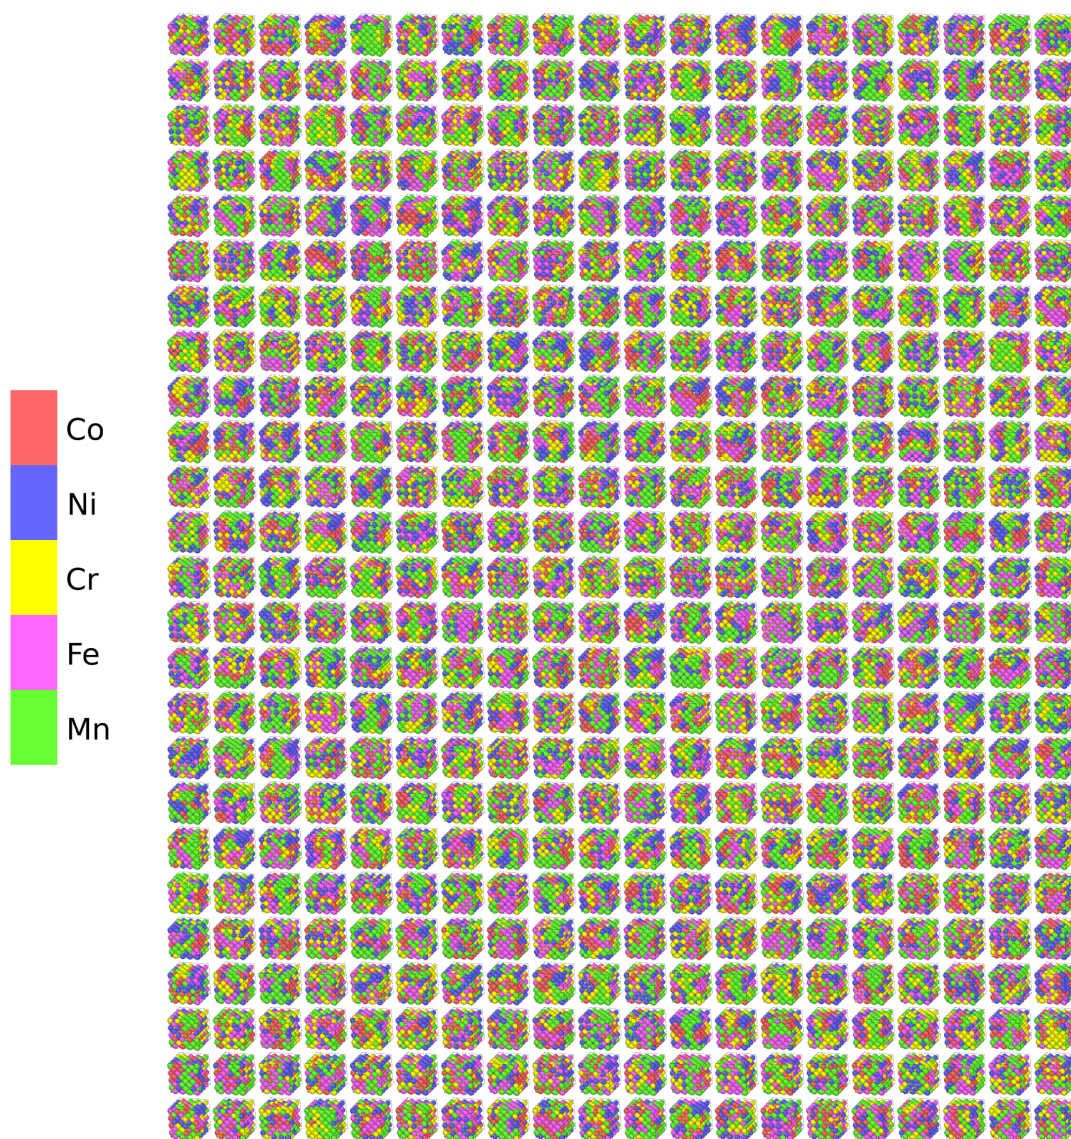

Figure 2: Full CoNiCrFeMn training set, generated via surrogate CE models.
